# Supplementary material for: The trans- and post-capture orbital evolution of Triton
Source: arXiv:2409.16983 source file (2024-09-25)
Supplement: Supplementary file 1 [file appendix_script.tex]

\chapter{A script}
\label{app:script}

\lstinputlisting{appendix/pythonscript.py}
%\label{app:code.infoblok}
